# Supplementary material for: 3D generation on ImageNet
Source: arXiv:2303.01416 source file (2023-03-02)
Supplement: Supplementary file 1 [file under-explored-ideas.tex]

\section{A list of under-explored ideas in our project}\label{ap:under-explored}

Our model consists on a lot of moving components
